# Supplementary material for: Data Formulator 2: Iterative Creation of Data Visualizations, with AI Transforming Data Along the Way
Source: arXiv:2408.16119 source file (2025-02-21)
Supplement: Supplementary file 1 [file 07-appendix.tex]

\section{Supplementary Materials}

Please check out our supplementary materials for (1) \df introduction video,  (2) unedited videos demonstrating \df's experiences to complete tasks in \autoref{sec:illustartive-scenarios} and user study tasks~\autoref{sec:evaluation}, and (3) user study handout.
